# Supplementary material for: Disentangling peri-urban river hypoxia
Source: arXiv:2510.05775 source file (2025-10-07)

# bgc total phytoplankton [mmol C m<sup>-3</sup>] in out

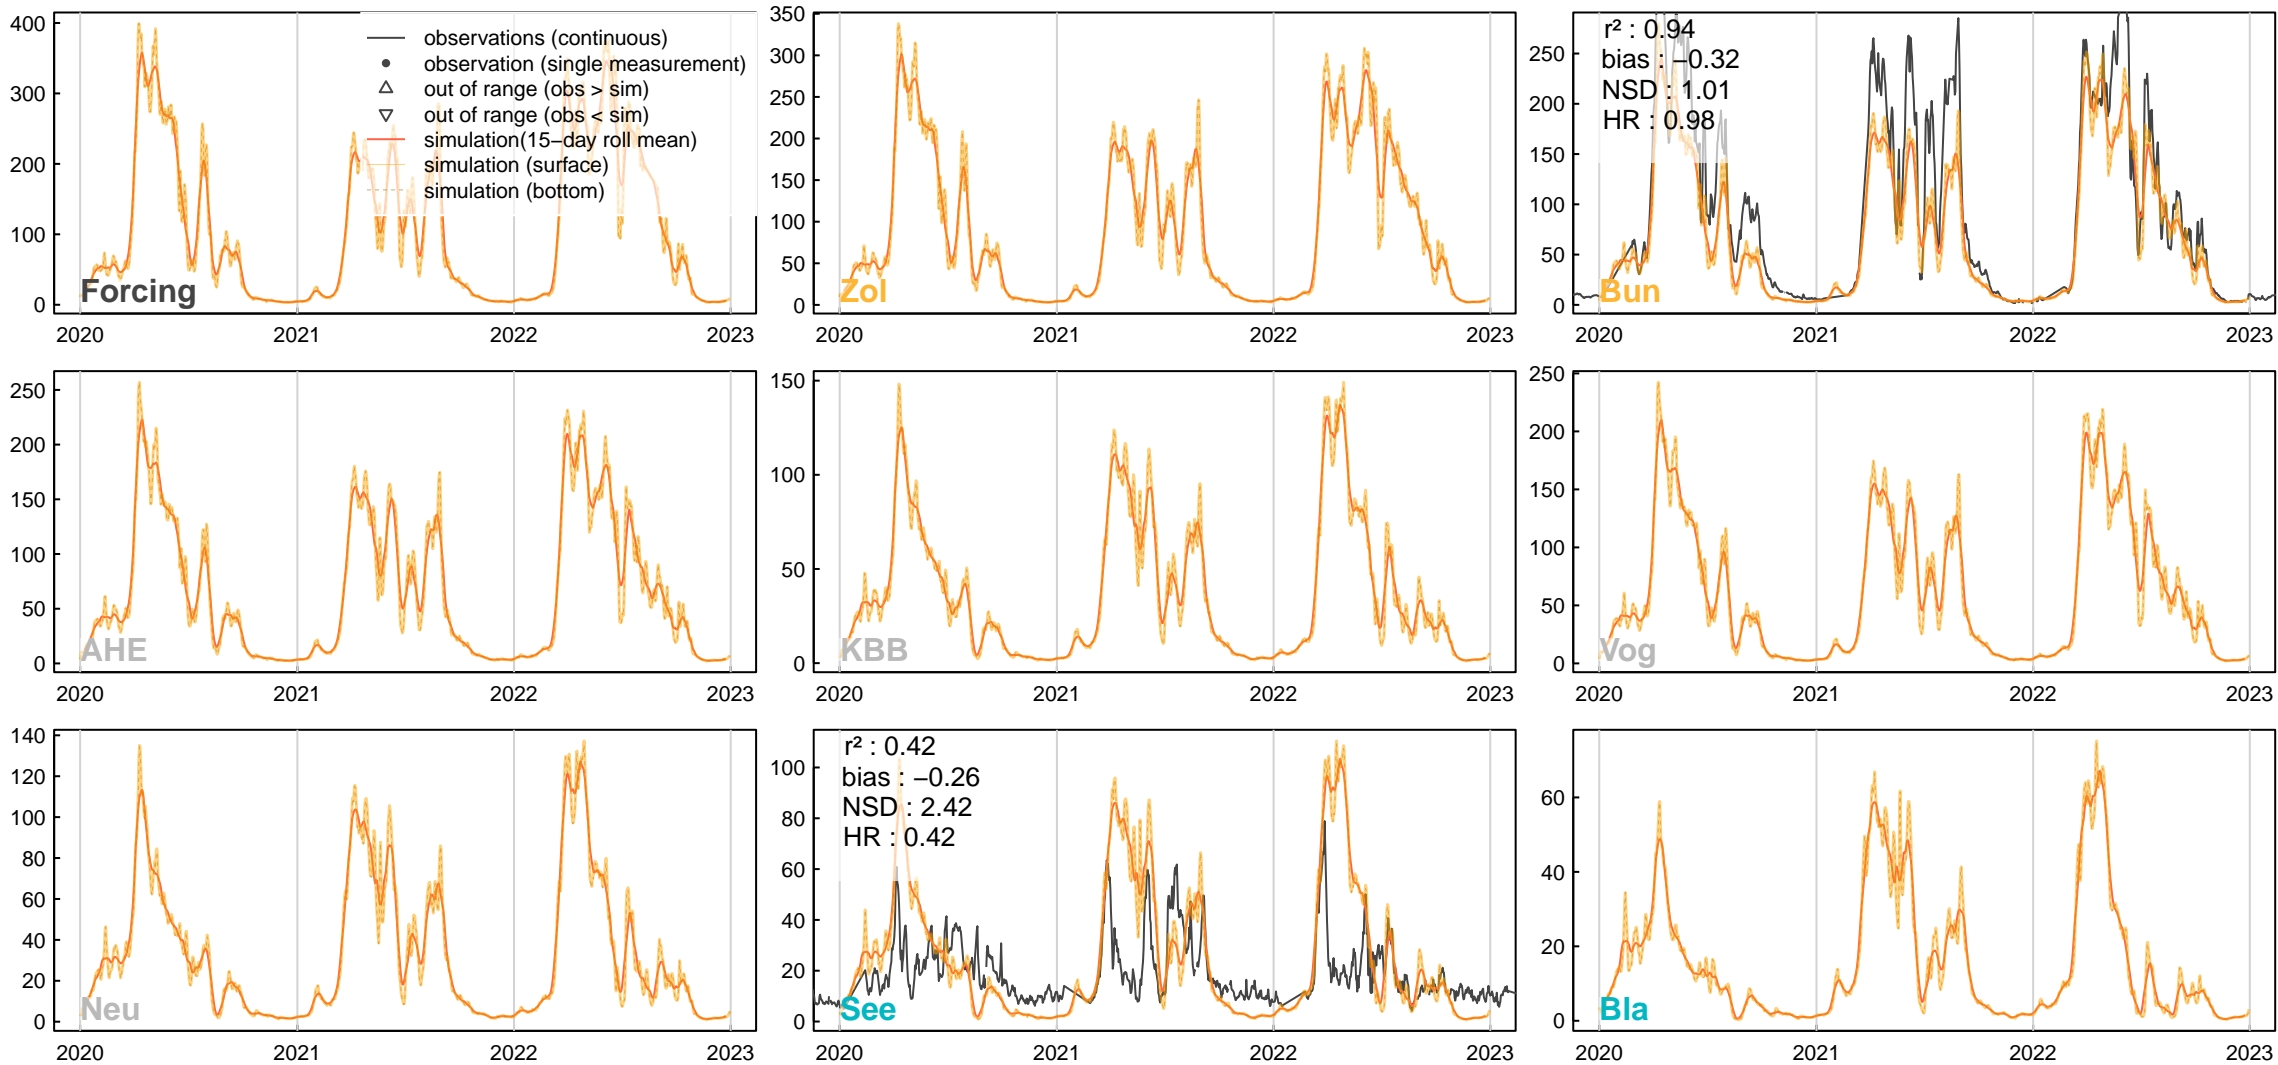

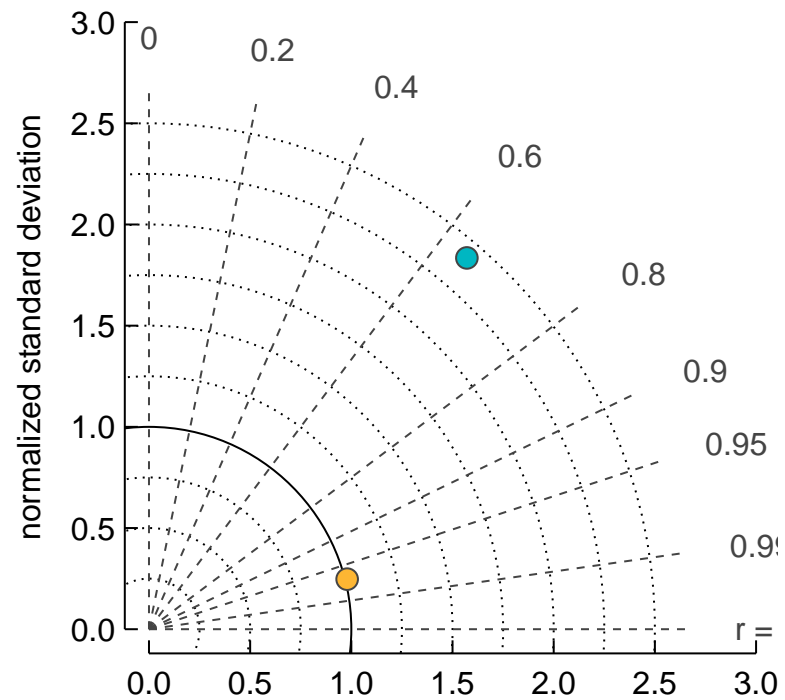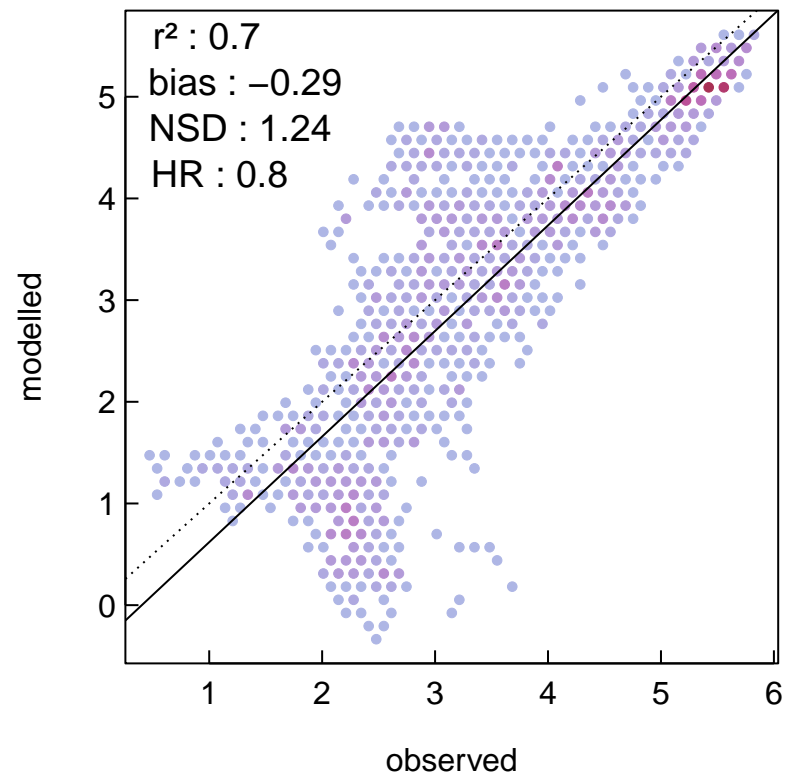

Supplement: Supplementary file 1 [file out.bgc_ALG.validation.pdf]
