# Supplementary material for: Disentangling peri-urban river hypoxia
Source: arXiv:2510.05775 source file (2025-10-07)

# bgc dissolved oxygen [mmol O<sub>2</sub> m<sup>-3</sup>] in out

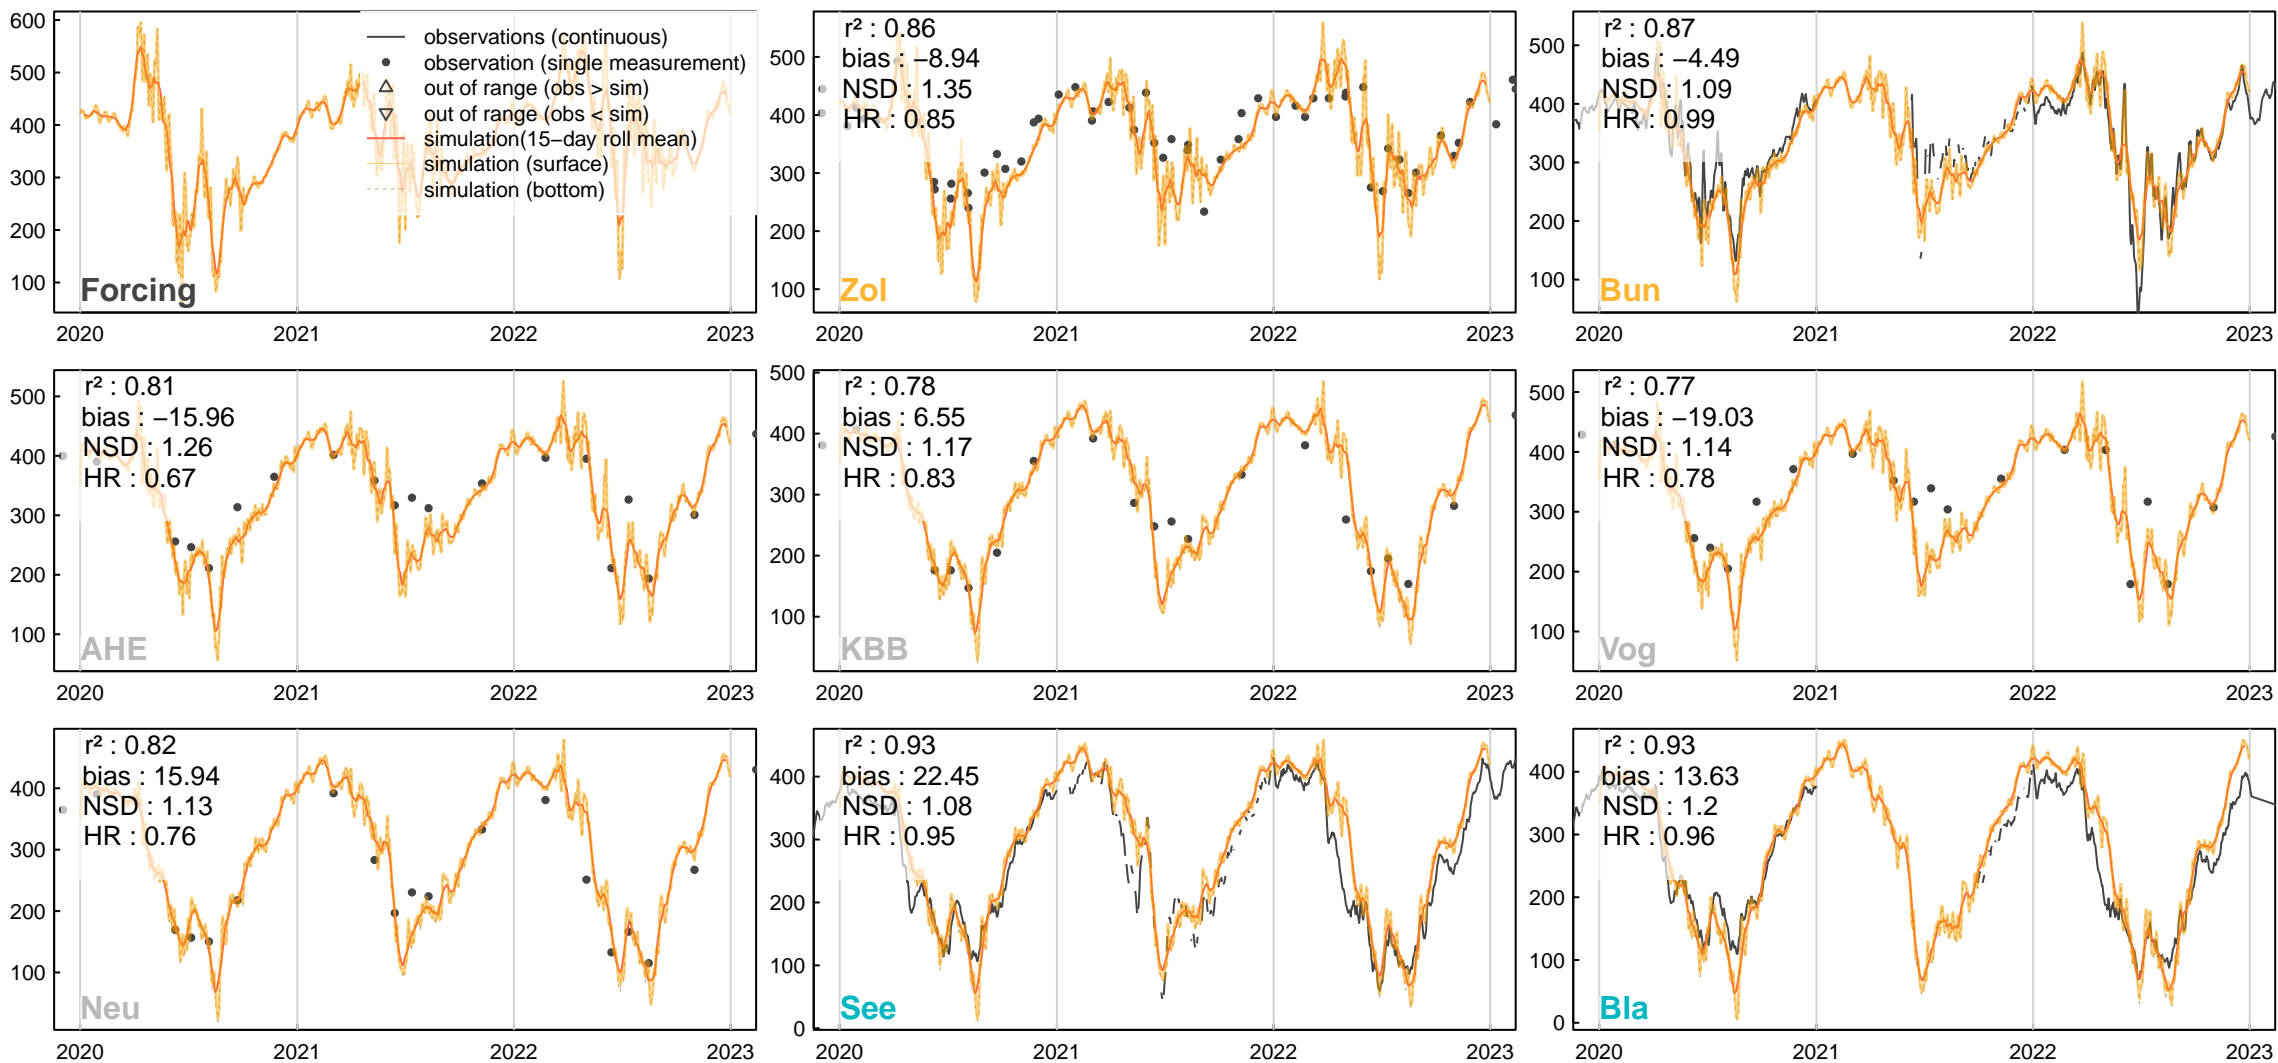

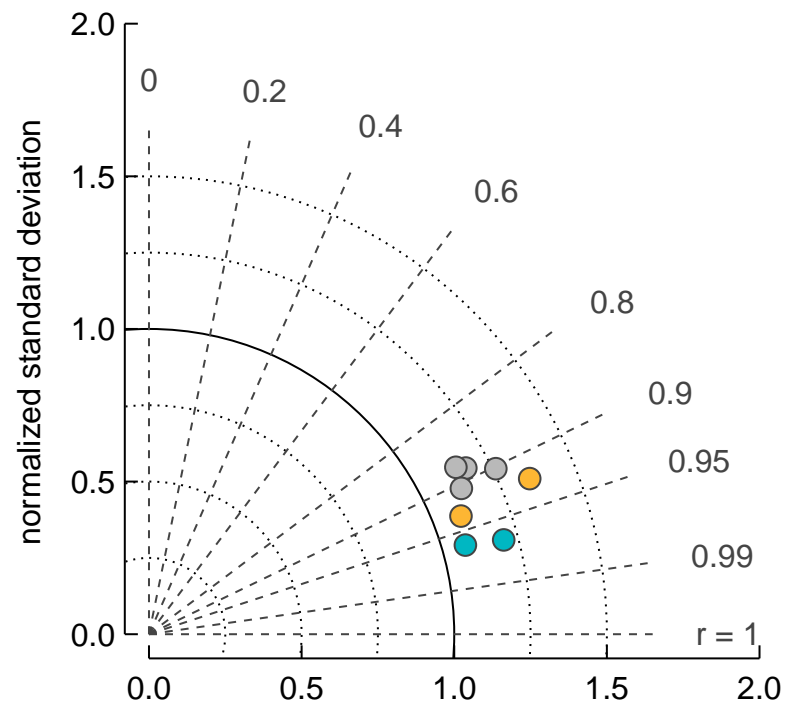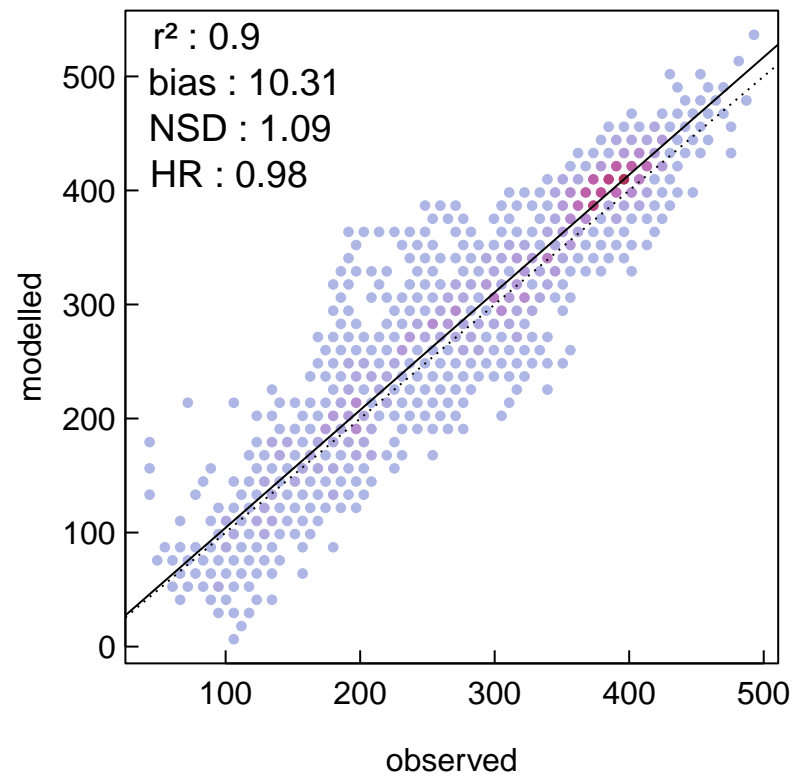

Supplement: Supplementary file 2 [file out.bgc_DOxy.validation.pdf]
