# Supplementary material for: Disentangling peri-urban river hypoxia
Source: arXiv:2510.05775 source file (2025-10-07)

# bgc nitrate [mmol N m<sup>-3</sup>] in out

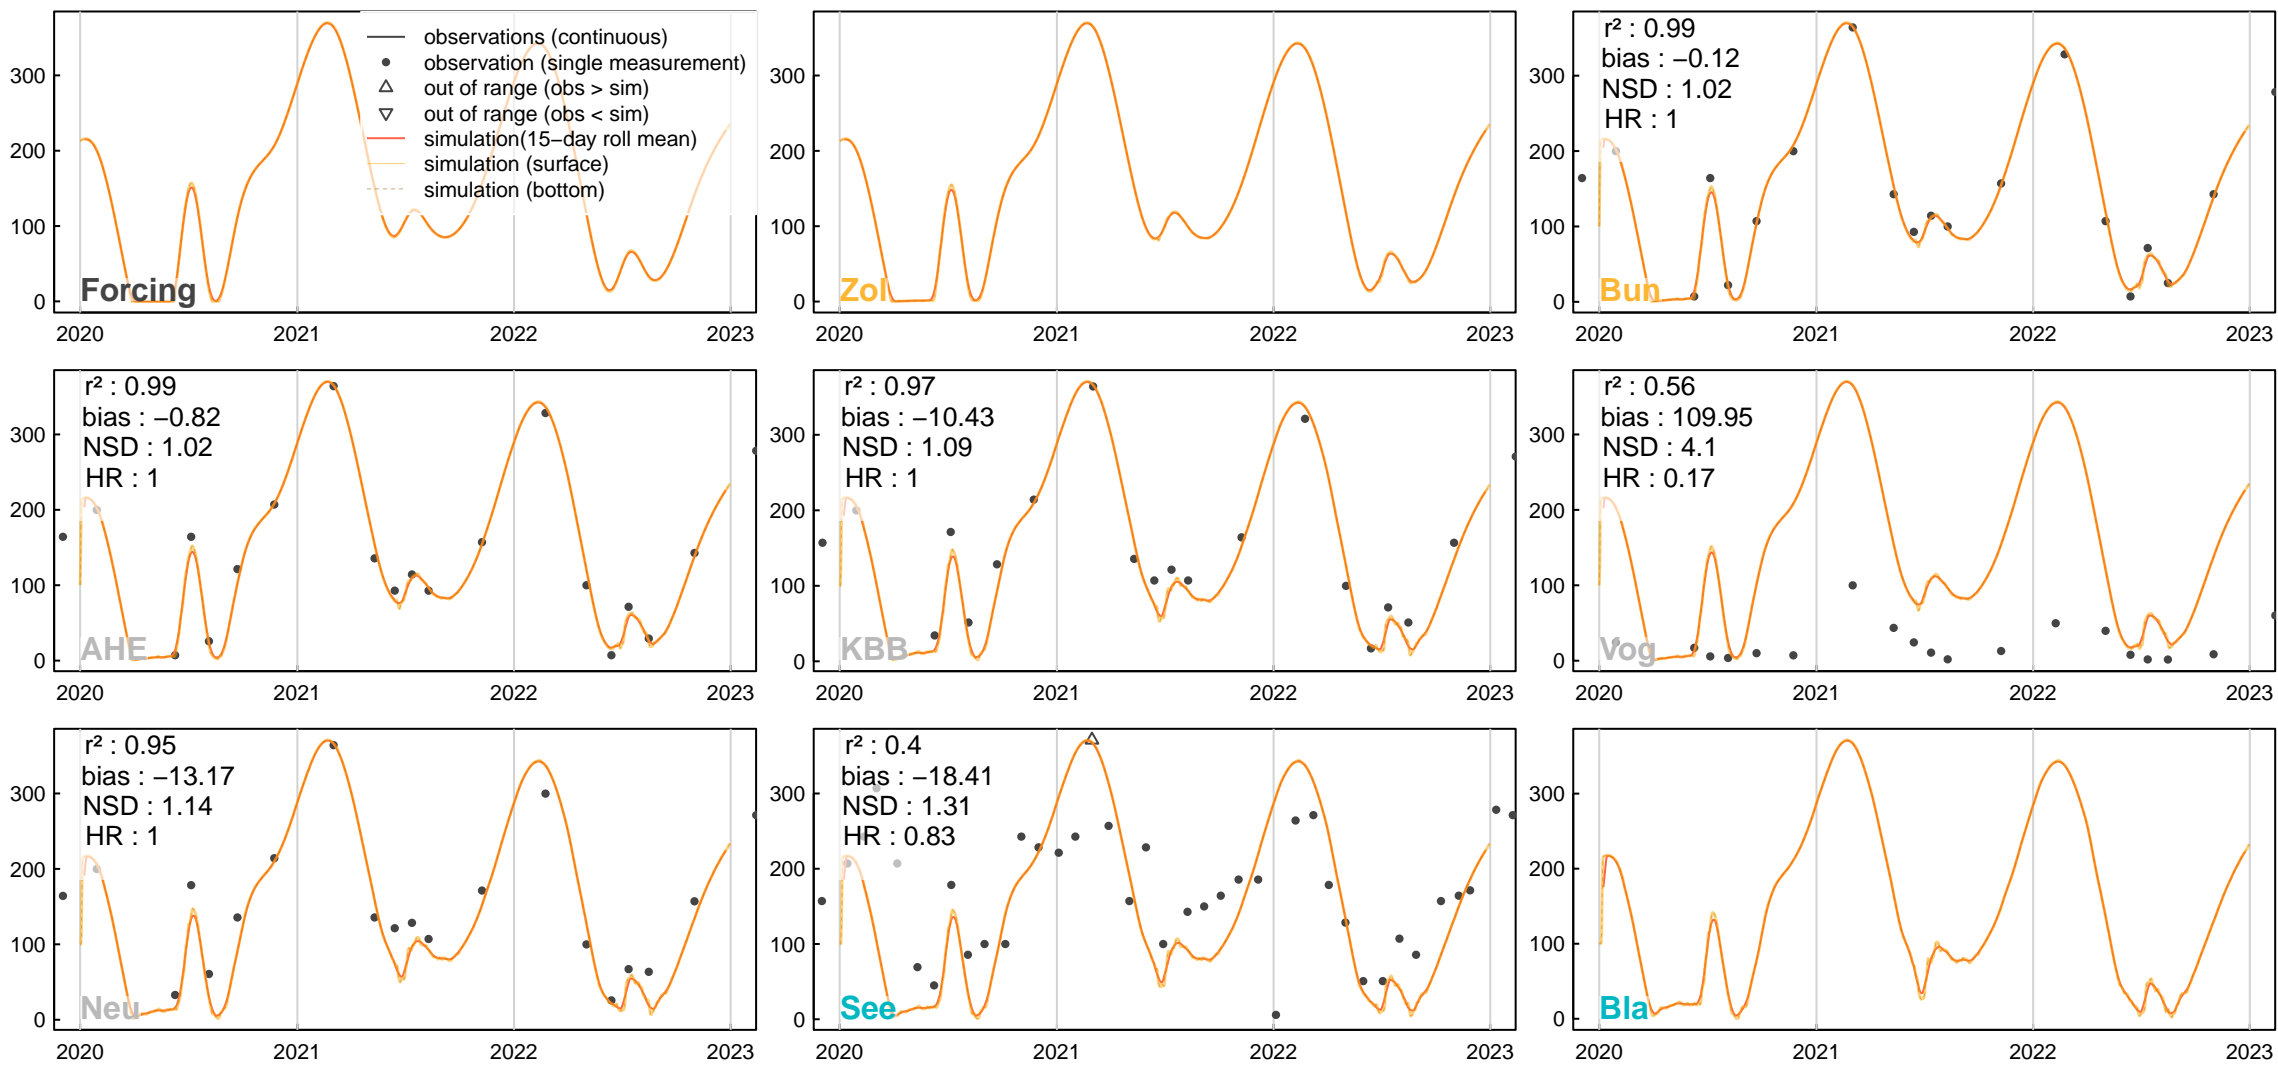

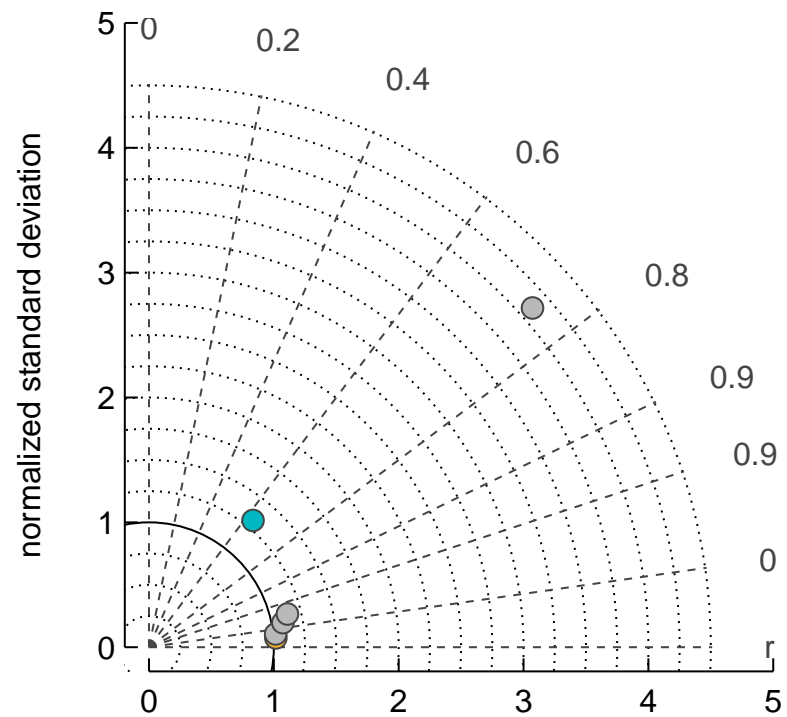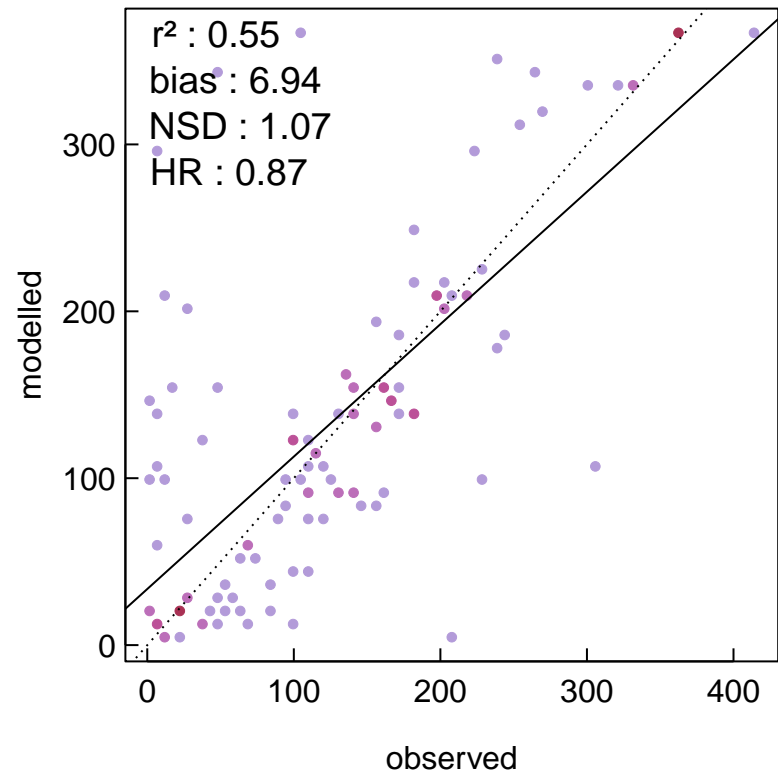

Supplement: Supplementary file 4 [file out.bgc_NO3.validation.pdf]
