# Supplementary material for: Disentangling peri-urban river hypoxia
Source: arXiv:2510.05775 source file (2025-10-07)

# bgc phosphate [mmol P m<sup>-3</sup>] in out

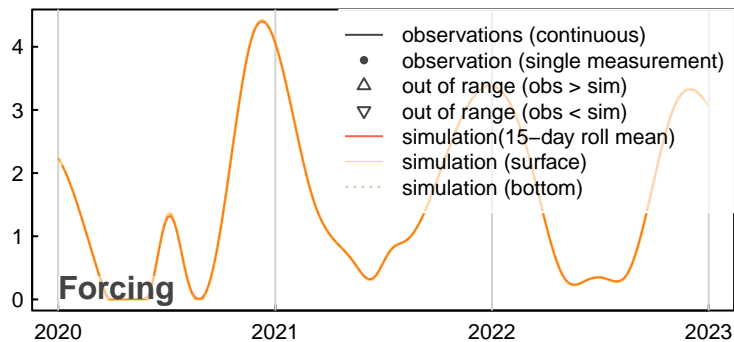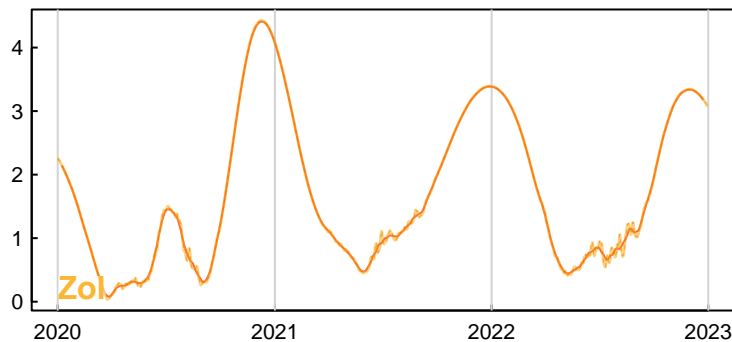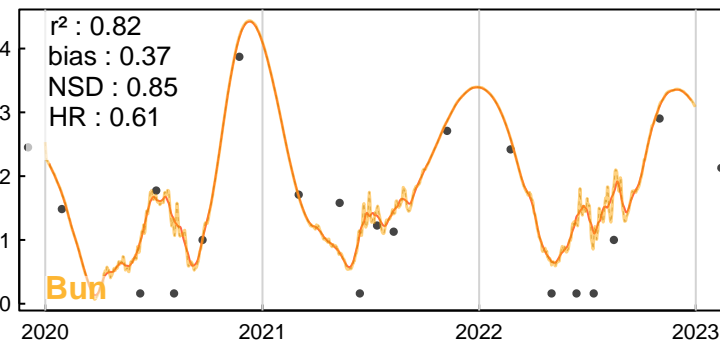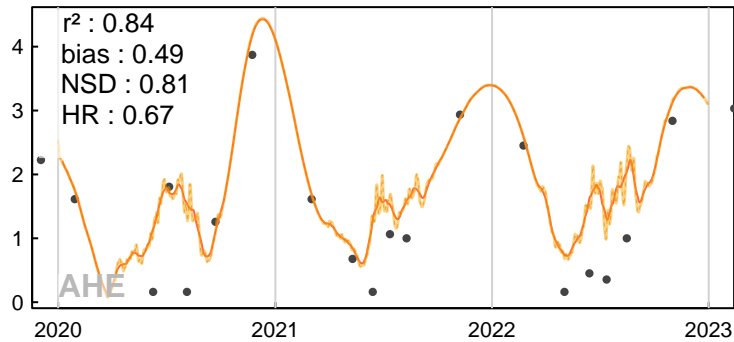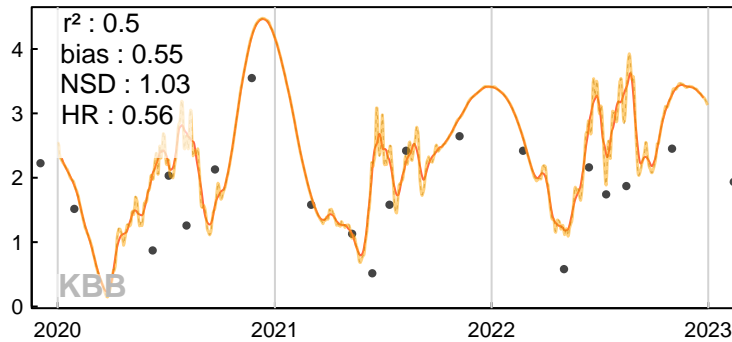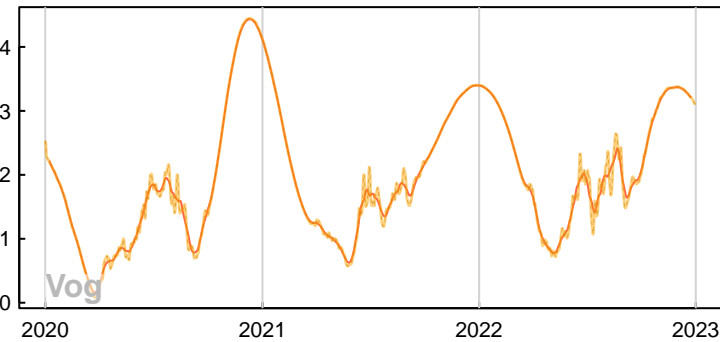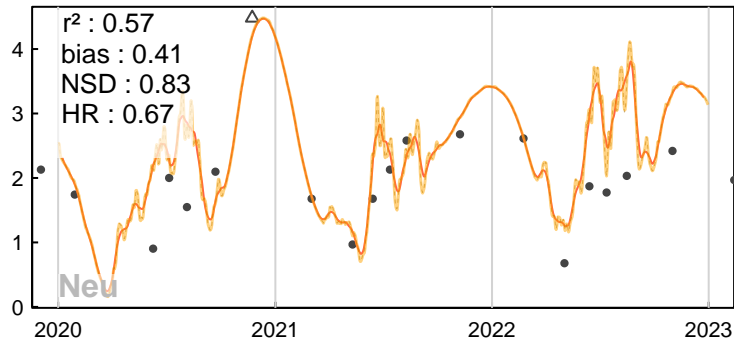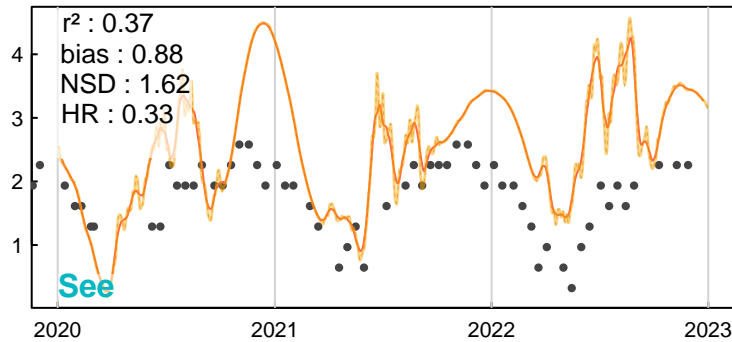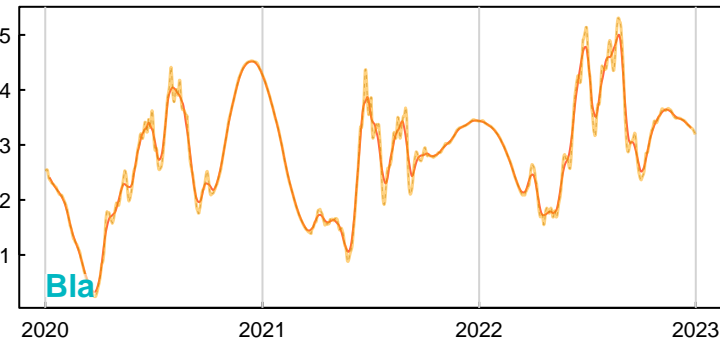

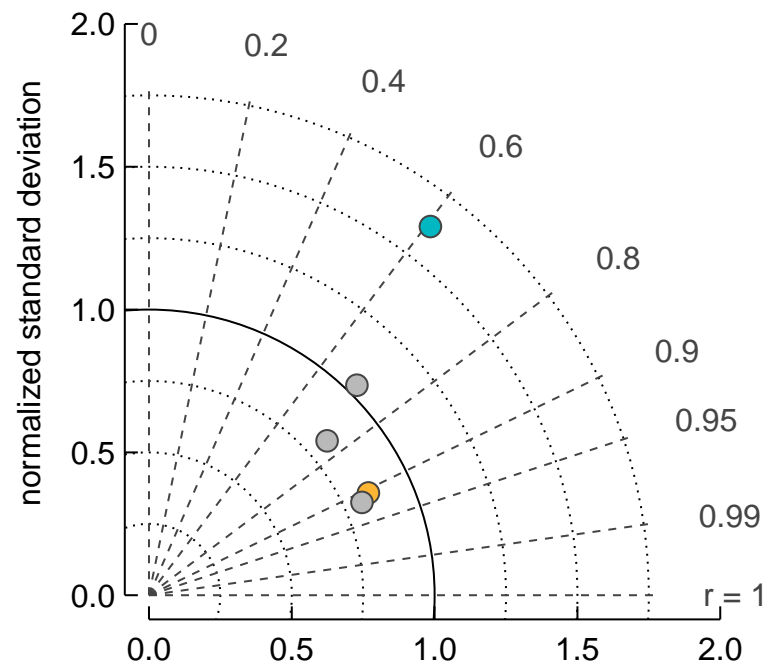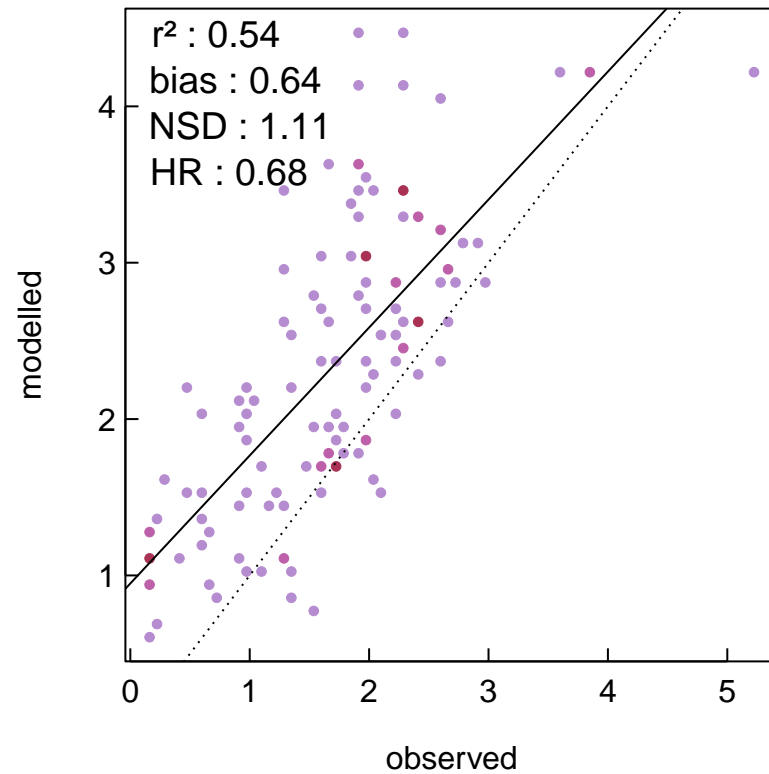

Supplement: Supplementary file 5 [file out.bgc_PO4.validation.pdf]
