# Supplementary material for: Disentangling peri-urban river hypoxia
Source: arXiv:2510.05775 source file (2025-10-07)

# temperature [Celsius] in out

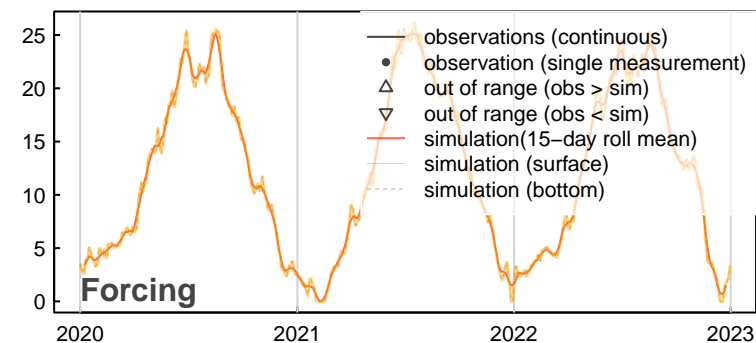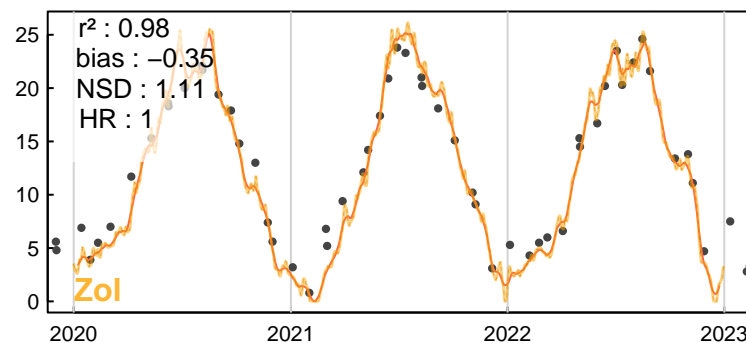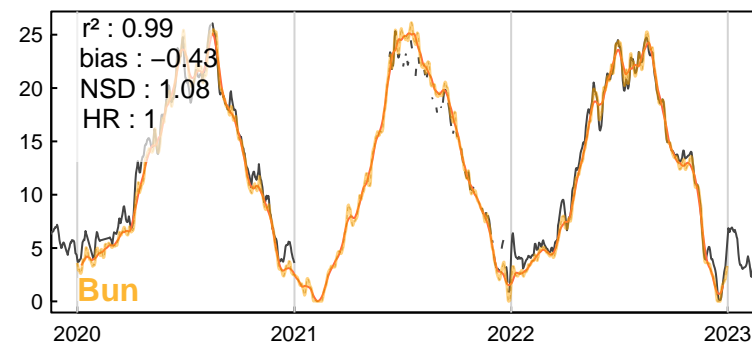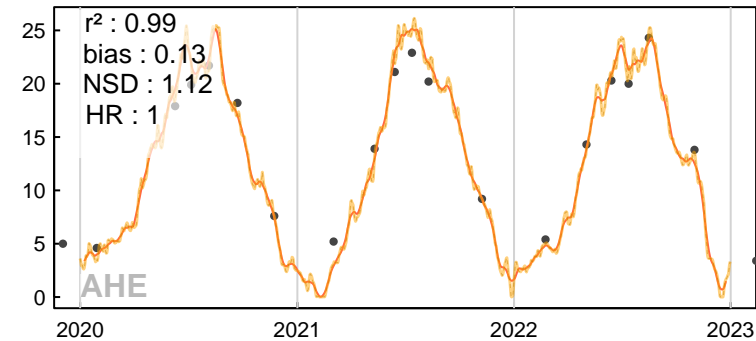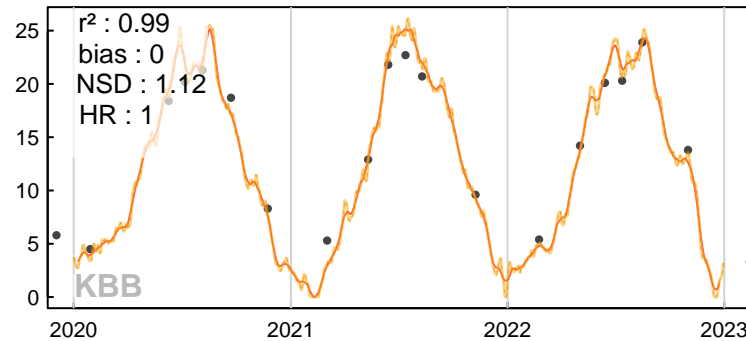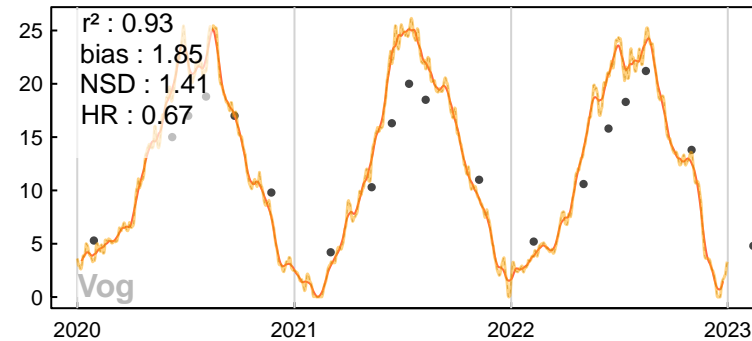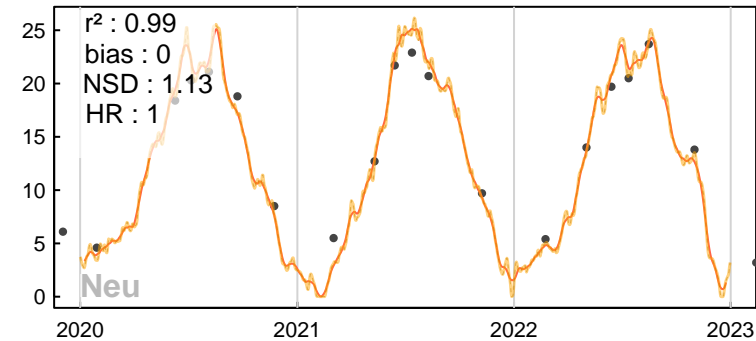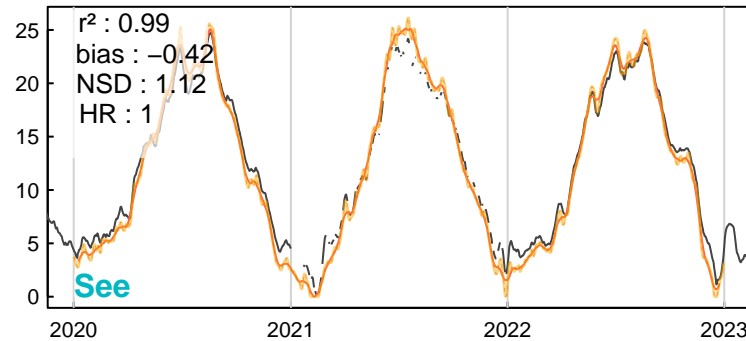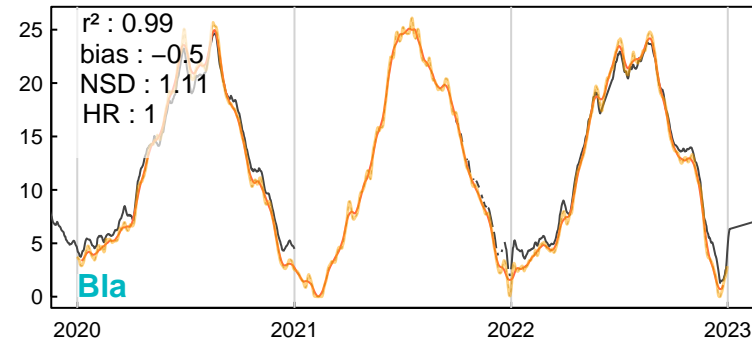

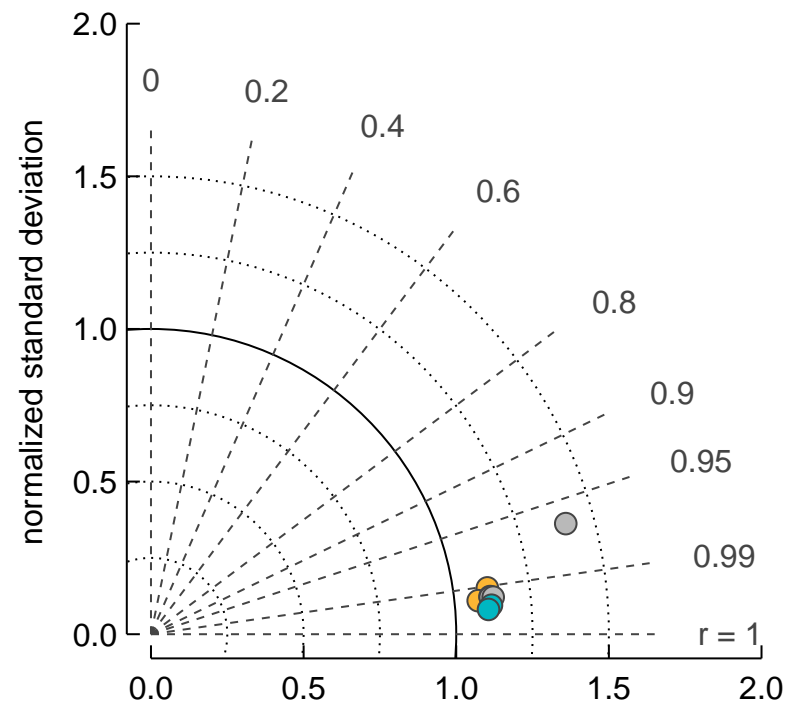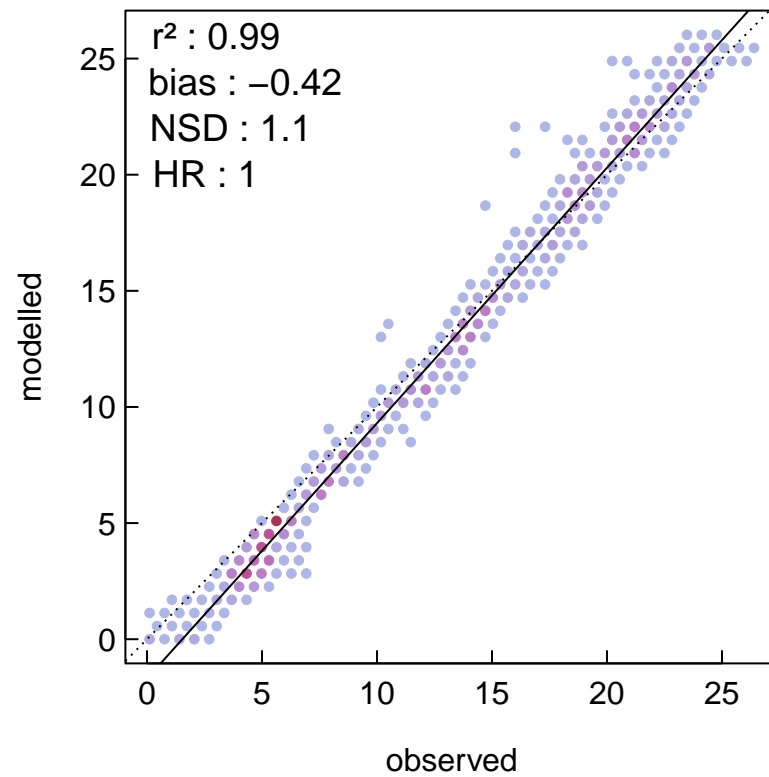

Supplement: Supplementary file 7 [file out.temp.validation.pdf]
